# Supplementary material for: Stellar photoionisation modelling in SYNTHESIZER
Source: arXiv:2607.27467 source file (2026-07-29)
Supplement: Supplementary file 1 [file appendix.tex]

\begin{appendix}

% \subsection{Currently available grids}\label{app:grids}

% \begin{table*}[t]
% \centering
% \caption{Currently available grids in \synthesizer.}
% \begin{tabular}{lcccccccc}
% \hline
% Column 1 & Column 2 & Column 3 & Column 4 & Column 5 & Column 6 & Column 7 & Column 8 & Column 9 \\
% \hline
% Row 1 & a & b & c & d & e & f & g & h \\
% Row 2 & i & j & k & l & m & n & o & p \\
% Row 3 & q & r & s & t & u & v & w & x \\
% Row 4 & y & z & aa & bb & cc & dd & ee & ff \\
% Row 5 & gg & hh & ii & jj & kk & ll & mm & nn \\
% \hline

% \hline
% \end{tabular}
% \label{tab:grids}
% \end{table*}

% \subsection{Reference Abundance Patterns}\label{sec:}

% \begin{figure}
%     \centering
%     \includegraphics[width=1\columnwidth]{figures/modelling/reference_abundance_patterns.pdf}
%     \caption{Reference abundance patterns currently available within \synthesizer.}
%     \label{fig:appendix:reference_abundance_patterns}
% \end{figure}

% \comment{Also provide a table}

\end{appendix}
